# Supplementary material for: Collective control of modular soft robots via embodied Spiking Neural Cellular Automata
Source: arXiv:2204.02099 source file (2022-04-05)
Supplement: Supplementary file 1 [file supplementary.tex]

\newpage

\section*{Supplementary material}

\begin{figure}[ht]
    \centering
    \begin{tikzpicture}
        \begin{groupplot}[
            boxplot,
            boxplot/draw direction=y,
            width=0.3\linewidth,
            height=0.35\linewidth,
            group style={
                group size=4 by 3,
                horizontal sep=1mm,
                vertical sep=1mm,
                xticklabels at=edge bottom,
                yticklabels at=edge left
            },
            ymin=-1,ymax=21,xticklabels=\empty,
            legend cell align={left}
        ]
            % biped
            \nextgroupplot[
                align=center,
                legend columns=3,
                legend entries={MLP,LIF-SNN,LIFH-SNN},
                title={CA-1},
                ylabel={$v_x$},
                legend to name=best
            ]
            % swap area legend with mark=* to have a circle
            \addlegendimage{mark=*,color=colorbrewer1,fill}
            \addlegendimage{mark=*,color=colorbrewer5,fill}
            \addlegendimage{mark=*,color=colorbrewer2,fill}
            
            \addplot[black, fill=colorbrewer1] table[y=MLP] {data/boxplot/b_biped_CA1.txt};
            \addplot[black, fill=colorbrewer5] table[y=LIF] {data/boxplot/b_biped_CA1.txt};
            \addplot[black, fill=colorbrewer2] table[y=LIF-H] {data/boxplot/b_biped_CA1.txt};
            
            \nextgroupplot[align=center,title={CA-4}]
            \addplot[black, fill=colorbrewer1] table[y=MLP] {data/boxplot/b_biped_CA4.txt};
            \addplot[black, fill=colorbrewer5] table[y=LIF] {data/boxplot/b_biped_CA4.txt};
            \addplot[black, fill=colorbrewer2] table[y=LIF-H] {data/boxplot/b_biped_CA4.txt};
            
            \nextgroupplot[align=center,title={Homo}]
            \addplot[black, fill=colorbrewer1] table[y=MLP] {data/boxplot/b_biped_homo.txt};
            \addplot[black, fill=colorbrewer5] table[y=LIF] {data/boxplot/b_biped_homo.txt};
            \addplot[black, fill=colorbrewer2] table[y=LIF-H] {data/boxplot/b_biped_homo.txt};
            
            \nextgroupplot[align=center,title={Hetero},ylabel={Biped}, yticklabel pos=right]
            \addplot[black, fill=colorbrewer1] table[y=MLP] {data/boxplot/b_biped_hetero.txt};
            \addplot[black, fill=colorbrewer5] table[y=LIF] {data/boxplot/b_biped_hetero.txt};
            \addplot[black, fill=colorbrewer2] table[y=LIF-H] {data/boxplot/b_biped_hetero.txt};
            
            % comb
            \nextgroupplot[ylabel={$v_x$}]
            \addplot[black, fill=colorbrewer1] table[y=MLP] {data/boxplot/b_comb_CA1.txt};
            \addplot[black, fill=colorbrewer5] table[y=LIF] {data/boxplot/b_comb_CA1.txt};
            \addplot[black, fill=colorbrewer2] table[y=LIF-H] {data/boxplot/b_comb_CA1.txt};
            
            \nextgroupplot
            \addplot[black, fill=colorbrewer1] table[y=MLP] {data/boxplot/b_comb_CA4.txt};
            \addplot[black, fill=colorbrewer5] table[y=LIF] {data/boxplot/b_comb_CA4.txt};
            \addplot[black, fill=colorbrewer2] table[y=LIF-H] {data/boxplot/b_comb_CA4.txt};
            
            \nextgroupplot
            \addplot[black, fill=colorbrewer1] table[y=MLP] {data/boxplot/b_comb_homo.txt};
            \addplot[black, fill=colorbrewer5] table[y=LIF] {data/boxplot/b_comb_homo.txt};
            \addplot[black, fill=colorbrewer2] table[y=LIF-H] {data/boxplot/b_comb_homo.txt};
            
            \nextgroupplot[ylabel={Comb}, yticklabel pos=right]
            \addplot[black, fill=colorbrewer1] table[y=MLP] {data/boxplot/b_comb_hetero.txt};
            \addplot[black, fill=colorbrewer5] table[y=LIF] {data/boxplot/b_comb_hetero.txt};
            \addplot[black, fill=colorbrewer2] table[y=LIF-H] {data/boxplot/b_comb_hetero.txt};
            
            % worm
            \nextgroupplot[ylabel={$v_x$}]
            \addplot[black, fill=colorbrewer1] table[y=MLP] {data/boxplot/b_worm_CA1.txt};
            \addplot[black, fill=colorbrewer5] table[y=LIF] {data/boxplot/b_worm_CA1.txt};
            \addplot[black, fill=colorbrewer2] table[y=LIF-H] {data/boxplot/b_worm_CA1.txt};
            
            \nextgroupplot
            \addplot[black, fill=colorbrewer1] table[y=MLP] {data/boxplot/b_worm_CA4.txt};
            \addplot[black, fill=colorbrewer5] table[y=LIF] {data/boxplot/b_worm_CA4.txt};
            \addplot[black, fill=colorbrewer2] table[y=LIF-H] {data/boxplot/b_worm_CA4.txt};
            
            \nextgroupplot
            \addplot[black, fill=colorbrewer1] table[y=MLP] {data/boxplot/b_worm_homo.txt};
            \addplot[black, fill=colorbrewer5] table[y=LIF] {data/boxplot/b_worm_homo.txt};
            \addplot[black, fill=colorbrewer2] table[y=LIF-H] {data/boxplot/b_worm_homo.txt};
            
            \nextgroupplot[ylabel={Worm}, yticklabel pos=right]
            \addplot[black, fill=colorbrewer1] table[y=MLP] {data/boxplot/b_worm_hetero.txt};
            \addplot[black, fill=colorbrewer5] table[y=LIF] {data/boxplot/b_worm_hetero.txt};
            \addplot[black, fill=colorbrewer2] table[y=LIF-H] {data/boxplot/b_worm_hetero.txt};
            
        \end{groupplot}
    \end{tikzpicture}
    \\
    \tikzexternaldisable\pgfplotslegendfromname{best}\tikzexternalenable
    \caption{Best. P-values missing.}
    \label{fig:best}
\end{figure}

\begin{figure}[ht]
    \centering
    \begin{tikzpicture}
        \begin{groupplot}[
            boxplot,
            boxplot/draw direction=y,
            width=0.3\linewidth,
            height=0.35\linewidth,
            group style={
                group size=4 by 3,
                horizontal sep=1mm,
                vertical sep=1mm,
                xticklabels at=edge bottom,
                yticklabels at=edge left
            },
            ymin=-1,ymax=20,xticklabels=\empty,
            legend cell align={left}
        ]
            % biped
            \nextgroupplot[
                align=center,
                legend columns=3,
                legend entries={MLP,LIF-SNN,LIFH-SNN},
                title={CA-1},
                ylabel={$v_x$},
                legend to name=validation
            ]
            % swap area legend with mark=* to have a circle
            \addlegendimage{mark=*,color=colorbrewer1,fill}
            \addlegendimage{mark=*,color=colorbrewer5,fill}
            \addlegendimage{mark=*,color=colorbrewer2,fill}
            
            \addplot[black, fill=colorbrewer1] table[y=MLP] {data/boxplot/v_biped_CA1.txt};
            \addplot[black, fill=colorbrewer5] table[y=LIF] {data/boxplot/v_biped_CA1.txt};
            \addplot[black, fill=colorbrewer2] table[y=LIF-H] {data/boxplot/v_biped_CA1.txt};
            
            \nextgroupplot[align=center,title={CA-4}]
            \addplot[black, fill=colorbrewer1] table[y=MLP] {data/boxplot/v_biped_CA4.txt};
            \addplot[black, fill=colorbrewer5] table[y=LIF] {data/boxplot/v_biped_CA4.txt};
            \addplot[black, fill=colorbrewer2] table[y=LIF-H] {data/boxplot/v_biped_CA4.txt};
            
            \nextgroupplot[align=center,title={Homo}]
            \addplot[black, fill=colorbrewer1] table[y=MLP] {data/boxplot/v_biped_homo.txt};
            \addplot[black, fill=colorbrewer5] table[y=LIF] {data/boxplot/v_biped_homo.txt};
            \addplot[black, fill=colorbrewer2] table[y=LIF-H] {data/boxplot/v_biped_homo.txt};
            
            \nextgroupplot[align=center,title={Hetero},ylabel={Biped}, yticklabel pos=right]
            \addplot[black, fill=colorbrewer1] table[y=MLP] {data/boxplot/v_biped_hetero.txt};
            \addplot[black, fill=colorbrewer5] table[y=LIF] {data/boxplot/v_biped_hetero.txt};
            \addplot[black, fill=colorbrewer2] table[y=LIF-H] {data/boxplot/v_biped_hetero.txt};
            
            % comb
            \nextgroupplot[ylabel={$v_x$}]
            \addplot[black, fill=colorbrewer1] table[y=MLP] {data/boxplot/v_comb_CA1.txt};
            \addplot[black, fill=colorbrewer5] table[y=LIF] {data/boxplot/v_comb_CA1.txt};
            \addplot[black, fill=colorbrewer2] table[y=LIF-H] {data/boxplot/v_comb_CA1.txt};
            
            \nextgroupplot
            \addplot[black, fill=colorbrewer1] table[y=MLP] {data/boxplot/v_comb_CA4.txt};
            \addplot[black, fill=colorbrewer5] table[y=LIF] {data/boxplot/v_comb_CA4.txt};
            \addplot[black, fill=colorbrewer2] table[y=LIF-H] {data/boxplot/v_comb_CA4.txt};
            
            \nextgroupplot
            \addplot[black, fill=colorbrewer1] table[y=MLP] {data/boxplot/v_comb_homo.txt};
            \addplot[black, fill=colorbrewer5] table[y=LIF] {data/boxplot/v_comb_homo.txt};
            \addplot[black, fill=colorbrewer2] table[y=LIF-H] {data/boxplot/v_comb_homo.txt};
            
            \nextgroupplot[ylabel={Comb}, yticklabel pos=right]
            \addplot[black, fill=colorbrewer1] table[y=MLP] {data/boxplot/v_comb_hetero.txt};
            \addplot[black, fill=colorbrewer5] table[y=LIF] {data/boxplot/v_comb_hetero.txt};
            \addplot[black, fill=colorbrewer2] table[y=LIF-H] {data/boxplot/v_comb_hetero.txt};
            
            % worm
            \nextgroupplot[ylabel={$v_x$}]
            \addplot[black, fill=colorbrewer1] table[y=MLP] {data/boxplot/v_worm_CA1.txt};
            \addplot[black, fill=colorbrewer5] table[y=LIF] {data/boxplot/v_worm_CA1.txt};
            \addplot[black, fill=colorbrewer2] table[y=LIF-H] {data/boxplot/v_worm_CA1.txt};
            
            \nextgroupplot
            \addplot[black, fill=colorbrewer1] table[y=MLP] {data/boxplot/v_worm_CA4.txt};
            \addplot[black, fill=colorbrewer5] table[y=LIF] {data/boxplot/v_worm_CA4.txt};
            \addplot[black, fill=colorbrewer2] table[y=LIF-H] {data/boxplot/v_worm_CA4.txt};
            
            \nextgroupplot
            \addplot[black, fill=colorbrewer1] table[y=MLP] {data/boxplot/v_worm_homo.txt};
            \addplot[black, fill=colorbrewer5] table[y=LIF] {data/boxplot/v_worm_homo.txt};
            \addplot[black, fill=colorbrewer2] table[y=LIF-H] {data/boxplot/v_worm_homo.txt};
            
            \nextgroupplot[ylabel={Worm}, yticklabel pos=right]
            \addplot[black, fill=colorbrewer1] table[y=MLP] {data/boxplot/v_worm_hetero.txt};
            \addplot[black, fill=colorbrewer5] table[y=LIF] {data/boxplot/v_worm_hetero.txt};
            \addplot[black, fill=colorbrewer2] table[y=LIF-H] {data/boxplot/v_worm_hetero.txt};
            
        \end{groupplot}
    \end{tikzpicture}
    \\
    \tikzexternaldisable\pgfplotslegendfromname{validation}\tikzexternalenable
    \caption{Validation. P-values missing.}
    \label{fig:validation}
\end{figure}

\subsection{Importance of the neural model}
\begin{figure}[ht]
    \centering
    \begin{tikzpicture}
        \def\ptopabove{21}
        \def\ptopbelow{19}
        \def\pbottomabove{-1.5}
        \def\pbottombelow{-3.5}
        \begin{groupplot}[
            boxplot,
            boxplot/draw direction=y,
            width=0.4\linewidth,
            height=0.5\linewidth,
            group style={
                group size=2 by 1,
                horizontal sep=1mm,
                vertical sep=1mm,
                xticklabels at=edge bottom,
                yticklabels at=edge left
            },
            ymin=-6,ymax=23,xticklabels=\empty,
            legend cell align={left}
        ]
            \nextgroupplot[
                align=center,
                legend columns=3,
                legend entries={{S-NCA (w/ hom.)}, {S-NCA (w/o hom.)}, {NCA}, {Evolution}, {Adaptation}},
                title={Biped},
                ylabel={$v_x$},
                legend to name=snca
            ]
            \addlegendimage{mark=*,color=colorbrewer1,fill}
            \addlegendimage{mark=*,color=colorbrewer2,fill}
            \addlegendimage{mark=*,color=colorbrewer3,fill}
            \addlegendimage{area legend,color=black,fill}
            \addlegendimage{area legend,color=black,fill,fill opacity=0.4}
            \boxplotcouple{data/boxplot/b_biped_CA4.txt}{data/boxplot/v_biped_CA4.txt}{LIF-H}{colorbrewer1};
            \boxplotcouple{data/boxplot/b_biped_CA4.txt}{data/boxplot/v_biped_CA4.txt}{LIF}{colorbrewer2};
            \boxplotcouple{data/boxplot/b_biped_CA4.txt}{data/boxplot/v_biped_CA4.txt}{MLP}{colorbrewer3};
            \pvalue{1}{5}{\ptopabove}{$0.089$}
            \pvalue{1}{3}{\ptopbelow}{$1$}
            \pvalue{3}{5}{\ptopbelow}{$<0.01$}
            \pvaluebelow{2}{6}{\pbottombelow}{$<0.01$}
            \pvaluebelow{2}{4}{\pbottomabove}{$0.912$}
            \pvaluebelow{4}{6}{\pbottomabove}{$<0.01$}
            
            \nextgroupplot[align=center,title={Comb}]
            \boxplotcouple{data/boxplot/b_comb_CA4.txt}{data/boxplot/v_comb_CA4.txt}{LIF-H}{colorbrewer1};
            \boxplotcouple{data/boxplot/b_comb_CA4.txt}{data/boxplot/v_comb_CA4.txt}{LIF}{colorbrewer2};
            \boxplotcouple{data/boxplot/b_comb_CA4.txt}{data/boxplot/v_comb_CA4.txt}{MLP}{colorbrewer3};
            \pvalue{1}{5}{\ptopabove}{$0.173$}
            \pvalue{1}{3}{\ptopbelow}{$0.122$}
            \pvalue{3}{5}{\ptopbelow}{$0.023$}
            \pvaluebelow{2}{6}{\pbottombelow}{$0.121$}
            \pvaluebelow{2}{4}{\pbottomabove}{$0.011$}
            \pvaluebelow{4}{6}{\pbottomabove}{$0.280$}
            
        \end{groupplot}
    \end{tikzpicture}
    \\
    \tikzexternaldisable\pgfplotslegendfromname{snca}\tikzexternalenable
    \caption{Further insight on the uniform non-directional case. Importance of homeostasis, and comparison of SNN with MLP.}
    \label{fig:unif-nondir}
\end{figure}

\subsection{Importance of the state size for non-directional NCA}\label{sec:state-size}
\begin{figure}[ht]
    \centering
    \begin{tikzpicture}
        \def\ptopabove{21}
        \def\ptopbelow{19}
        \def\pbottomabove{-1.5}
        \def\pbottombelow{-3.5}
        \begin{groupplot}[
            boxplot,
            boxplot/draw direction=y,
            width=0.4\linewidth,
            height=0.5\linewidth,
            group style={
                group size=2 by 1,
                horizontal sep=1mm,
                vertical sep=1mm,
                xticklabels at=edge bottom,
                yticklabels at=edge left
            },
            ymin=-3,ymax=21,xticklabels=\empty,
            legend cell align={left}
        ]
            \nextgroupplot[
                align=center,
                legend columns=2,
                legend entries={$n_c=4$, $n_c=1$, {Evolution}, {Adaptation}},
                title={Biped},
                ylabel={$v_x$},
                legend to name=ca14
            ]
            \addlegendimage{mark=*,color=colorbrewer1,fill}
            \addlegendimage{mark=*,color=colorbrewer2,fill}
            \addlegendimage{area legend,color=black,fill}
            \addlegendimage{area legend,color=black,fill,fill opacity=0.4}
            \boxplotcouple{data/boxplot/b_biped_CA4.txt}{data/boxplot/v_biped_CA4.txt}{LIF-H}{colorbrewer1};
            \boxplotcouple{data/boxplot/b_biped_CA1.txt}{data/boxplot/v_biped_CA1.txt}{LIF}{colorbrewer2};
            \pvalue{1}{3}{\ptopbelow}{$0.035$}
            \pvaluebelow{2}{4}{\pbottomabove}{$0.123$}
            
            \nextgroupplot[align=center,title={Comb}]
            \boxplotcouple{data/boxplot/b_comb_CA4.txt}{data/boxplot/v_comb_CA4.txt}{LIF-H}{colorbrewer1};
            \boxplotcouple{data/boxplot/b_comb_CA1.txt}{data/boxplot/v_comb_CA1.txt}{LIF}{colorbrewer2};
            \pvalue{1}{3}{\ptopbelow}{$0.083$}
            \pvaluebelow{2}{4}{\pbottomabove}{$0.026$}
            
        \end{groupplot}
    \end{tikzpicture}
    \\
    \tikzexternaldisable\pgfplotslegendfromname{ca14}\tikzexternalenable
    \caption{Importance of state size (always S-NCA with homeostasis).}
    \label{fig:ca4-ca1}
\end{figure}
